# Supplementary material for: Quantitative predictions of thermodynamic hysteresis: Temperature-dependent character of the phase transition in Pd-H
Source: arXiv:2110.07883 ancillary file (2021-10-15)
Supplement: Supplementary file 1 [file supporting-information.pdf]

Supporting Information

# Quantitative predictions of thermodynamic hysteresis: Temperature-dependent character of the phase transition in Pd–H

J. Magnus Rahm, Joakim Löfgren, and Paul Erhart

## Contents

**Notes** **2**

SN1. Performance of the cluster expansion . . . 2
SN2. Calculation of interface energies . . . 2
SN3. Calculation of strain energy in arbitrary crystal directions . . . 2

**Figures** **4**

S1. ECIs and performance of the CE. . . . 4
S2. Excess strain energies and superlattice energies. . . . 4
S3. Distribution of atomic layer concentrations . . . 5
S4. Hysteresis in experiments on Pd nanocubes . . . 5
S5. Calculation of interface energies. . . . 6
S6. Lattice parameter in Pd–H . . . 6
S7. Elastic constants in Pd–H . . . 7
S8. Conversion from chemical potential to pressure . . . 7

**References** **8**

# Notes

## Supplementary Note 1: Performance of the cluster expansion

The cluster expansion (CE) fitted as described in the method section of the main paper has a cross-validation error over the training set (338 structures) of 1.0 meV/f.u. (formula unit = 1 H + 1 Pd), and root-mean-square error over the test set (30 structures) of 0.8 meV/f.u. The largest effective cluster interaction (ECI) (except zerolet and singlet) is obtained for the second nearest neighbor pair (Figure S1a) and all triplet ECIs are smaller than 0.5 meV/f.u. (Figure S1b). The correlation between target and predicted mixing energies is very good (Figure S1c, $R^2 = 0.98$), and the CE captures the energetics well over the entire concentration range (Figure S1d). In particular, the positive mixing energy in the H-poor limit (which is partially responsible for the two-phase region) is captured satisfactorily.

Having established the performance of the CE for small, single-phase structures, we now assess the impact of strain. The $\Delta E_{\mathrm{CS}}(\hat{\boldsymbol{k}}, c)$ term, defined in Eq. (6) of the main paper and calculated with density-functional theory (DFT), is the lowest for {100} interfaces and highest for {111} (Figure S2a). This indicates that strain favors {100} interfaces. To ensure that our CE reproduces DFT results for configurations with a high degree of strain, we calculated the energy of {100}, {110}, and {111} superlattices, having $n$ atomic planes fully occupied by hydrogen and $n$ unoccupied, periodically alternating. Our CE generally reproduces the DFT energies for these structures well (Figure S2b–d). Of course, such structures are thermodynamically unfavorable, since the hydrogen occupation in the $\beta$ phase is far below 100% for any reasonable hydrogen pressure. To obtain a thermodynamically relevant model we need to sample the CE model with Monte Carlo (MC) simulations.

## Supplementary Note 2: Calculation of interface energies

The most common approach for calculating the interface free energy between two phases $\alpha$ and $\beta$ using atomistic simulations is to compute the (free) energy difference between systems with and without interfaces,

$$\gamma_{\alpha/\beta}(\hat{\boldsymbol{k}}) = \frac{F_{\alpha/\beta}(c_{\mathrm{av}}, \hat{\boldsymbol{k}}) - V_\alpha f_\alpha(c_\alpha) - V_\beta f_\beta(c_\beta)}{2A}, \tag{1}$$

where $F_{\alpha/\beta}(c_{\mathrm{av}}, \hat{\boldsymbol{k}})$ is the free energy of the phase-separated system at overall concentration $c_{\mathrm{av}}$ with interface orientation $\hat{\boldsymbol{k}}$, $f_\alpha(c_\alpha)$ and $f_\beta(c_\beta)$ are the free energies per volume of the constituent phases at their respective concentrations, $V_\alpha$ and $V_\beta$ are the volumes of the two phases (directly related to $c_{\mathrm{av}}$, $c_\alpha$, and $c_\beta$), and $A$ is the cross section of the simulation cell. In the coherent case, this formula is not easily applicable, because the reference states $f_\alpha(c_\alpha)$ and $f_\beta(c_\beta)$ need to be taken as the strained phases. While these can in principle be calculated, great care needs to be applied to ensure the correct lattice parameter and the correct concentrations (which, as we have seen, typically deviate from both the incoherent and the coherent phase boundary concentration), and Eq. (1) is in practice highly vulnerable to noise in these reference calculations. When using a CE with constituent strain, these challenges can in principle be avoided as one can explicitly remove the strain term from $F_{\alpha/\beta}(c_{\mathrm{av}}, \hat{\boldsymbol{k}})$ and use unstrained reference energies for $f_\alpha(c_\alpha)$ and $f_\beta(c_\beta)$, which is possible since strain is an explicit term in this model. Nevertheless, we have found that this approach is still very sensitive to the numerical quality in the reference calculations, which always contain some degree of noise from MC sampling, as well as an uncertainty in the concentrations $c_\alpha$ and $c_\beta$ of the two phases.

An alternative approach, previously applied to surface energy calculations via DFT (1, 2), is to extrapolate the (free) energy to the limit of zero atomic layers,

$$\gamma_{\alpha/\beta}(\hat{\boldsymbol{k}}) = \lim_{N \to 0} \frac{F_{\alpha/\beta}(c_{\mathrm{av}}, \hat{\boldsymbol{k}}, N)}{2A}, \tag{2}$$

where $F_{\alpha/\beta}(c_{\mathrm{av}}, \hat{\boldsymbol{k}}, N)$ is the free energy obtained from a MC simulation with $N$ atomic layers in the simulation cell. We calculate the area $A$ using a lattice parameter fitted to the overall concentration using the DFT calculations of the training structures (Figure S6). Then, using a linear fit to $(N, F_{\alpha/\beta}(c_{\mathrm{av}}, \hat{\boldsymbol{k}}, N))$ data for increasing $N$ (Figure S5a), we obtain interface energies that are insensitive to noise in the MC sampling and stable over the concentration regime of the two-phase region (Figure S5b).

## Supplementary Note 3: Calculation of strain energy in arbitrary crystal directions

The constituent strain energy term, $E_{\mathrm{CS}}(\hat{\boldsymbol{k}}, c)$ depends on crystal direction $\hat{\boldsymbol{k}}$. Since it is multiplied by the structure factor $S(\boldsymbol{k}, \sigma)$ (see Eq. (7) of the main paper), it is for a given supercell not necessary to know $E_{\mathrm{CS}}(\hat{\boldsymbol{k}}, c)$ for any arbitrary direction, but only those directions for which there is a $\boldsymbol{k}$-point with a corresponding

nonzero structure factor. It can be shown that only integer multiples of the lattice vectors of the reciprocal cell of the superlattice yield nonzero structure factors (3). Yet, if we want to apply the approach to many different supercell shapes, the number of directions $\hat{\boldsymbol{k}}$ in which we need to know $E_{\mathrm{CS}}(\hat{\boldsymbol{k}}, c)$ becomes large. Since a large number of DFT calculations are required for each such direction, in practice, it is necessary to calculate $E_{\mathrm{CS}}(\hat{\boldsymbol{k}}, c)$ for a limited number of directions and obtain others by interpolation.

To this end, we first fitted Redlich–Kister polynomials to $E_{\mathrm{CS}}(\hat{\boldsymbol{k}}, c)$,

$$E_{\mathrm{CS}}(\hat{\boldsymbol{k}}, c) = c(1-c) \sum_{p=0}^{4} L_p(\hat{\boldsymbol{k}})(1-2c)^p, \tag{3}$$

which can be done with essentially no loss of accuracy, since the original data is very smooth. We thus obtained five expansion coefficients $L_p(\hat{\boldsymbol{k}})$ for each of the six crystal directions considered ($\langle 100\rangle$, $\langle 111\rangle$, $\langle 110\rangle$, $\langle 210\rangle$, $\langle 221\rangle$, $\langle 311\rangle$). Using the normalized corresponding vectors $\hat{\boldsymbol{k}}$, we made a least-squares fit of each Redlich–Kister coefficient $L_p(\hat{\boldsymbol{k}})$ to the functional form

$$L_p(\hat{\boldsymbol{k}}) = a_0 + a_1 k_y + a_2 k_z + a_3 k_y^2 + a_4 k_z^2 + a_5 k_y k_z \tag{4}$$

(using $\hat{\boldsymbol{k}}$ in the irreducible Brillouin zone defined by $k_x \geq k_y \geq k_z \geq 0$). Since the number of expansion coefficients in this expression is the same as the number of available values of $L_p(\hat{\boldsymbol{k}})$, this fit reproduces the known Redlich–Kister coefficients exactly. Using the parameters obtained by these two fits, we can evaluate $E_{\mathrm{CS}}(\hat{\boldsymbol{k}}, c)$ in an arbitrary direction $\hat{\boldsymbol{k}}$ using first Eq. (4) and then Eq. (3).

## Figures

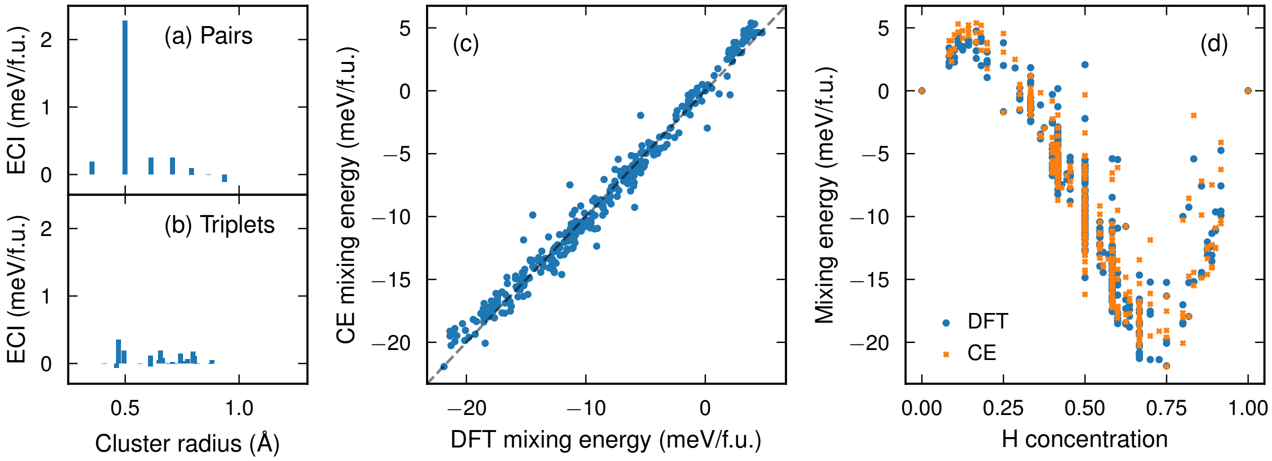


**Figure S1:** (a–b) ECIs of the CE developed in this work, for (a) pairs and (b) triplets. Not shown are the zerolet (11.2 meV/f.u.) and the singlet (26.4 meV/f.u.), which were constrained such that the energies at $c = 0$ and $c = 1$ are reproduced exactly. (c) Parity plot for all structures included in the fitting, exhibiting strong correlation ($R^2 = 0.98$). (d) Mixing energies are consequently reproduced well. Note in particular the positive mixing energy in the H-poor limit and the asymmetrically positioned minimum, together giving rise to a miscibility gap between $c = 0$ and $c \approx 2/3$ (at zero temperature). All energies are expressed per formula unit (1 formula unit = 1 H + 1 Pd)

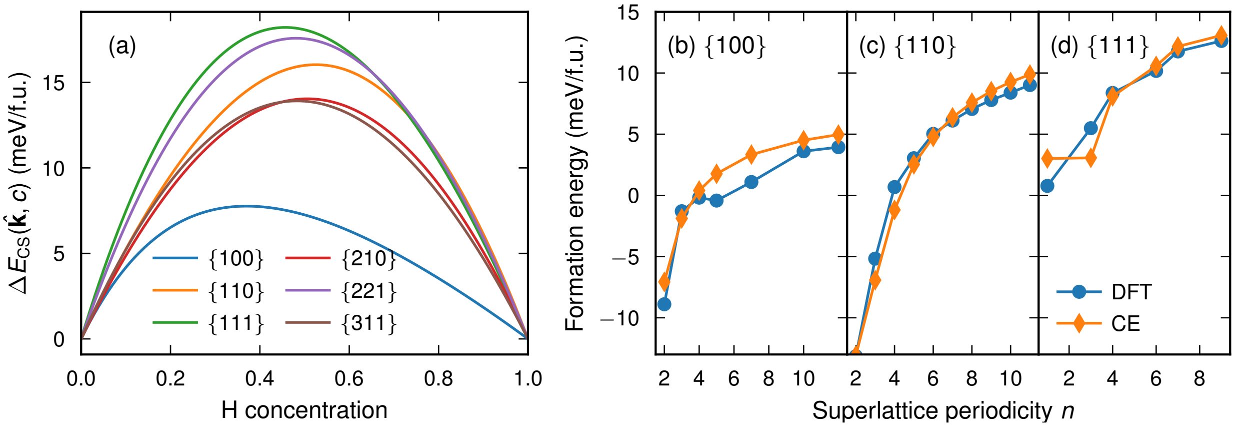


**Figure S2:** (a) The excess strain energy $\Delta E_{CS}(\hat{\boldsymbol{k}}, c)$ defined in Eq. (6) of the main paper and calculated with DFT. The strain is smallest for $\hat{\boldsymbol{k}} = (1, 0, 0)$ and largest for $\hat{\boldsymbol{k}} = (1, 1, 1)$. (b–d) Performance of the CE for the formation energies (= mixing energy) of superlattices of increasing periodicity $n$ ($n$ being the number of fully occupied atomic layers) in the (b) {100}, (c) {110}, and (d) {111} direction. DFT energies (blue lines) are compared to the prediction by our CE (orange lines).

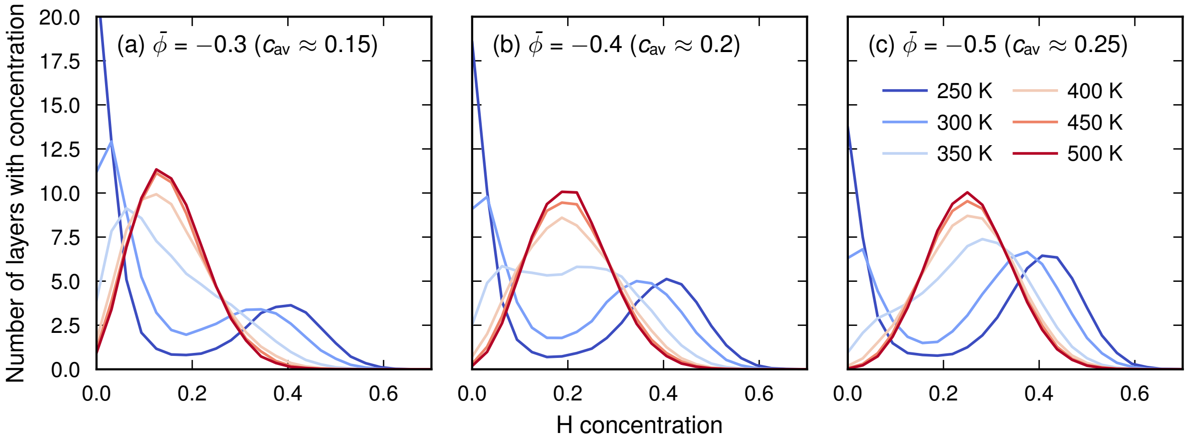


**Figure S3:** Distribution of concentrations per atomic layer in a $4 \times 4 \times 35$ supercell, using (a) $\bar{\phi} = -0.3$, (b) $\bar{\phi} = -0.4$ and (c) $\bar{\phi} = -0.5$, corresponding approximately to overall concentrations $c_{\text{av}} \approx 0.15$, 0.2 and 0.25, respectively. The data has been generated by calculating the concentration in each of the 70 atomic layers at every $N$-th interval ($N$ being the number of sites in the cell), and averaging over all such snapshots. At low temperatures ($\leq 300\,\text{K}$), there are two distinct peaks, one close to $c = 0$, and one at $c \approx 0.4$. At 350 K, the peaks are close to merging into one, and at 400 K and above, only one peak can be discerned. This behavior is consistent with the closing of the coherent two-phase region at approximately 400 K, as discussed in the main paper.

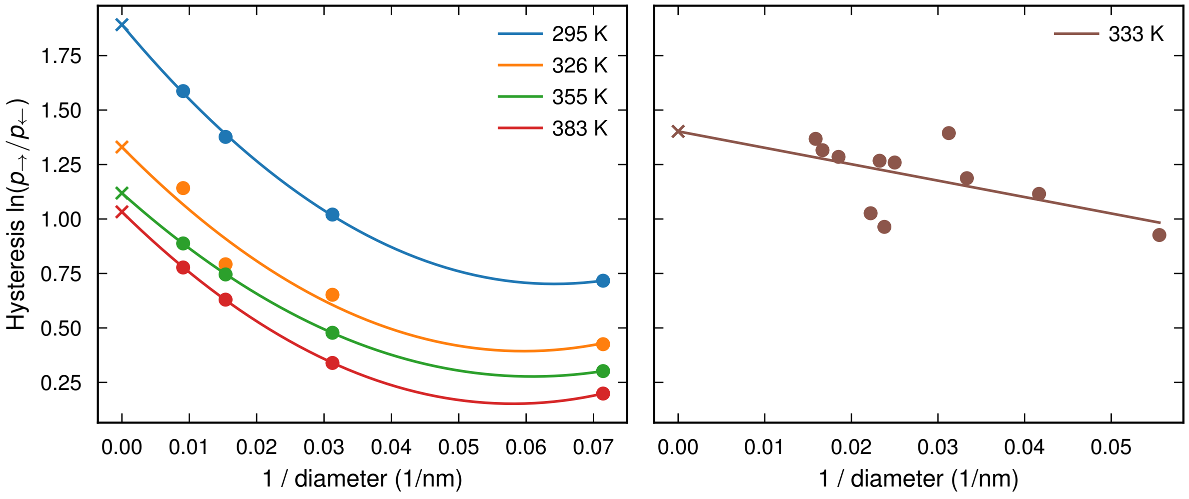


**Figure S4:** Hysteresis between absorption and desorption of hydrogen in Pd nanocubes, from (a) Bardhan *et al.* (4) (ensemble measurements) and (b) Syrenova *et al.* (5) (single-particle measurements). The hysteresis is size-dependent, and to make the data comparable to the bulk limit where our model is valid, we extrapolate the hysteresis. In (a), the data is fairly consistent, and we find that a two-degree polynomial fits the data well. In the single-particle data of (b), data points are more scattered and we use a linear fit. The data marked by crosses, indicating where the fits intercept the $y$ axis, were used for experimental comparisons in the main paper.

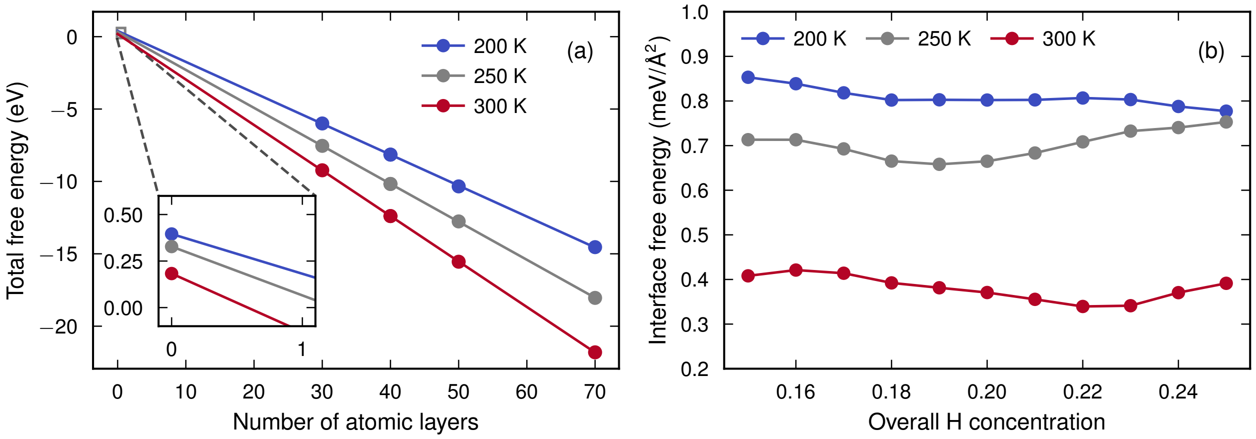


**Figure S5:** Calculation of interface energies, in the present case for {100} interfaces. (a) By extrapolation of a linear fit of free energies as a function of the number of atomic layers to the limit of zero layers (inset), the interface energy can be calculated from the intercept using Eq. (2). The results are based on calculations at an overall hydrogen concentration of 0.2. (b) The results are relatively constant as a function of overall concentration.

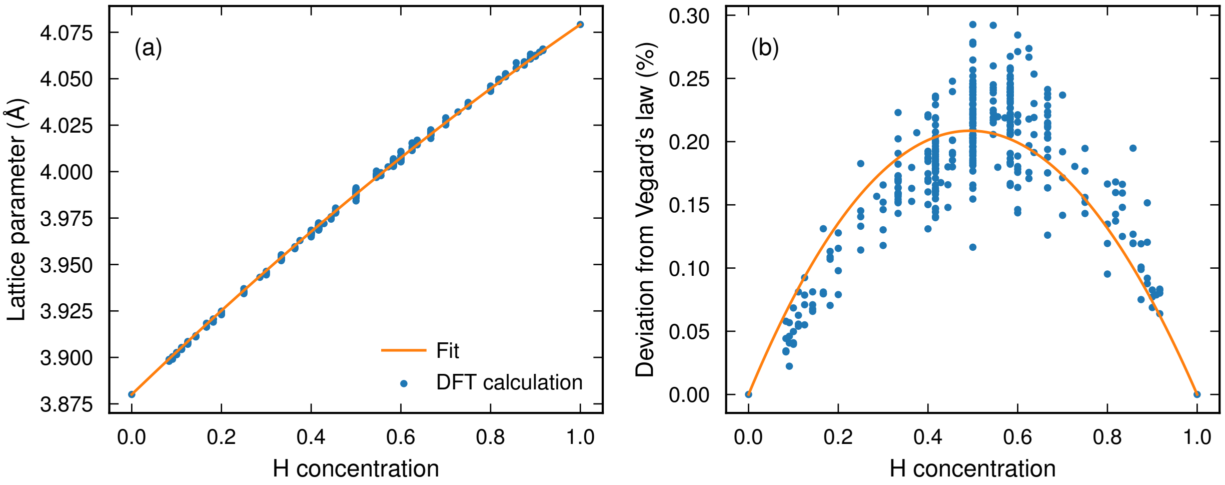


**Figure S6:** Lattice parameter in Pd–H from DFT calculations for different hydrogen concentrations and configurations. (a) The variation with composition is linear to a first approximation. (b) By plotting the relative deviation of the lattice parameter from a weighted average of the lattice parameters of Pd and PdH with 100% H, a small but significant deviation from Vegard's law is apparent. The concentration dependence of the lattice parameter can be well reproduced by a fit to the functional form $a(c) = (1-c)a_{\mathrm{Pd}} + ca_{\mathrm{PdH}} + Ac(1-c)$, where $a_{\mathrm{Pd}} = 3.8800$ Å, $a_{\mathrm{PdH}} = 4.0792$ Å, and $A = 0.0332$ Å (orange lines).

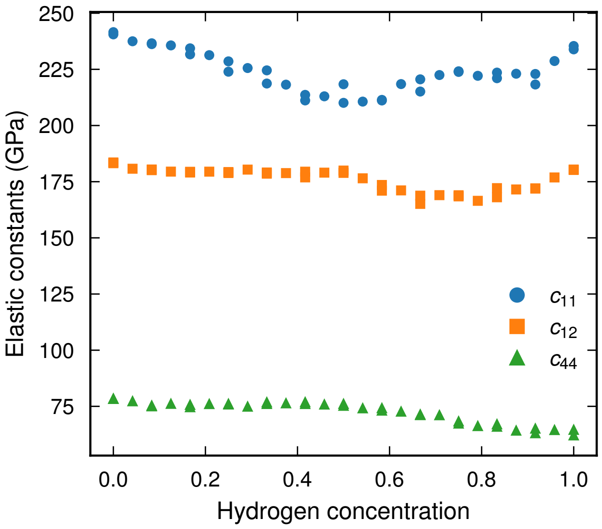


**Figure S7:** Elastic constants in Pd–H as a function of H content, calculated with DFT using special quasirandom structures (6).

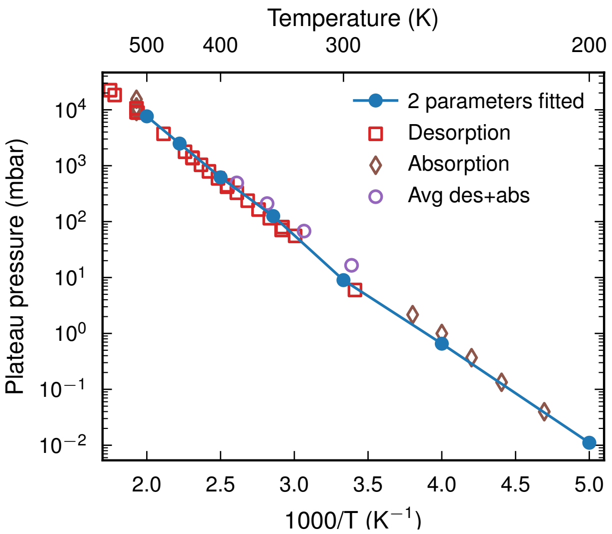


**Figure S8:** Plateau pressure in absorption and desorption isotherms of hydrogen in pure Pd. Red squares, brown diamonds and purple circles are, respectively, experimental desorption, absorption and average desorption/absorption pressures from the literature (4, 7–10). Blue dots mark the plateau pressures obtained with our CE model using a two-parameter fit to convert $\bar{\mu}$ to $H_2$ hydrogen pressure, specifically $P = \exp[(2\bar{\mu}+p(T))/k_\mathrm{B}T]$, with $p(T) = 1.2\,\mathrm{meV/K} \cdot T - 0.368\,\mathrm{eV}$.

# References


[1] J. C. Boettger, *Nonconvergence of surface energies obtained from thin-film calculations,* Physical Review B **49**, 16798 (1994). doi:10.1103/PhysRevB.49.16798.

[2] V. Fiorentini and M. Methfessel, *Extracting convergent surface energies from slab calculations,* Journal of Physics: Condensed Matter **8**, 6525 (1996). doi:10.1088/0953-8984/8/36/005.

[3] D. B. Laks, L. G. Ferreira, S. Froyen, and A. Zunger, *Efficient cluster expansion for substitutional systems,* Physical Review B **46**, 12587 (1992). doi:10.1103/PhysRevB.46.12587.

[4] R. Bardhan, L. O. Hedges, C. L. Pint, A. Javey, S. Whitelam, and J. J. Urban, *Uncovering the intrinsic size dependence of hydriding phase transformations in nanocrystals,* Nature Materials **12**, 905 (2013). doi:10.1038/nmat3716.

[5] S. Syrenova, C. Wadell, F. A. Nugroho, T. A. Gschneidtner, Y. A. D. Fernandez, G. Nalin, D. Świtlik, F. Westerlund, T. J. Antosiewicz, V. P. Zhdanov, *et al.*, *Hydride formation thermodynamics and hysteresis in individual Pd nanocrystals with different size and shape,* Nature Materials **14**, 1236 (2015). doi:10.1038/nmat4409.

[6] A. Zunger, S. H. Wei, L. G. Ferreira, and J. E. Bernard, *Special quasirandom structures,* Physical Review Letters **65**, 353 (1990). doi:10.1103/PhysRevLett.65.353.

[7] H. Frieske and E. Wicke, *Magnetic Susceptibility and Equilibrium Diagram of* $PdH_n$*,* Berichte der Bunsengesellschaft für physikalische Chemie **77**, 48 (1973). doi:10.1002/bbpc.19730770112.

[8] R. Lässer and K. H. Klatt, *Solubility of hydrogen isotopes in palladium,* Physical Review B **28**, 748 (1983). doi:10.1103/PhysRevB.28.748.

[9] C. Picard, O. J. Kleppa, and G. Boureau, *A thermodynamic study of the palladium–hydrogen system at 245–352°C and at pressures up to 34 atm,* The Journal of Chemical Physics **69**, 5549 (1978). doi:10.1063/1.436550.

[10] T. B. Flanagan and D. Wang, *Low temperature hydrogen and deuterium isotherms for Pd and some of its binary alloys,* Journal of Alloys and Compounds , 157434 (2020). doi:10.1016/j.jallcom.2020.157434.
